# Supplementary material for: ReTabAD: A Benchmark for Restoring Semantic Context in Tabular Anomaly Detection
Source: arXiv:2510.02060 source file (2026-05-28)
Supplement: Supplementary file 1 [file computation.tex]

\section{Computational Cost}
