# Supplementary material for: ReTabAD: A Benchmark for Restoring Semantic Context in Tabular Anomaly Detection
Source: arXiv:2510.02060 source file (2026-05-28)
Supplement: Supplementary file 2 [file ethics.tex]

% \section*{Ethics Statement}
% This work utilizes several publicly available healthcare datasets (e.g., cardiotocography, cirrhosis, glioma) that contain sensitive clinical information. 
% We emphasize that all experiments are conducted strictly for research purposes and do not involve direct patient interaction. 
% While our benchmark and methods are designed to advance anomaly detection research, false alarms in healthcare applications may lead to unnecessary interventions, patient anxiety, or resource misallocation. 
% Therefore, the models and results reported here should not be interpreted as ready for clinical deployment. 
% Any practical adoption in healthcare settings must be accompanied by rigorous validation, ethical review, and close collaboration with medical professionals.
