# Supplementary material for: ReTabAD: A Benchmark for Restoring Semantic Context in Tabular Anomaly Detection
Source: arXiv:2510.02060 source file (2026-05-28)
Supplement: Supplementary file 3 [file auprc_full_backup.tex]

\begin{table}[htbp]
\centering
\scriptsize
\caption{AUPRC Performance across all baselines.}
\label{tab:auprc_results2}
\resizebox{\textwidth}{!}{%
\begin{tabular}{lcccccccccccccccc}
\toprule
Dataset & OCSVM & LOF & KNN & IForest & PCA & DeepSVDD & REPEN & RDP & RCA & GOAD & NeuTraL & SLAD & DIF & MCM & DRL & AnoLLM \\
\midrule
\midrule
automobile & 0.578 & 0.618 & 0.534 & 0.543 & 0.419 & 0.762 & 0.496 & 0.637 & 0.566 & 0.620 & 0.718 & 0.665 & 0.544 & 0.675 & 0.661 & 0.553 \\
 & (±0.039) & (±0.031) & (±0.017) & (±0.039) & (±0.040) & (±0.065) & (±0.043) & (±0.049) & (±0.035) & (±0.094) & (±0.021) & (±0.060) & (±0.029) & (±0.038) & (±0.069) & (±0.025)\\

backdoor & 0.043 & 0.052 & 0.092 & 0.032 & 0.019 & 0.131 & 0.168 & 0.276 & 0.054 & 0.245 & 0.908 & 0.867 & 0.494 & 0.188 & 0.132 & 0.319 \\
 & (±0.002) & (±0.006) & (±0.005) & (±0.001) & (±0.000) & (±0.039) & (±0.011) & (±0.007) & (±0.003) & (±0.027) & (±0.000) & (±0.003) & (±0.044) & (±0.029) & (±0.033) &  (±0.012)\\

campaign & 0.539 & 0.524 & 0.572 & 0.559 & 0.580 & 0.561 & 0.523 & 0.517 & 0.560 & 0.563 & 0.593 & 0.563 & 0.507 & 0.588 & 0.561 & 0.573 \\
 & (±0.007) & (±0.004) & (±0.009) & (±0.010) & (±0.005) & (±0.013) & (±0.013) & (±0.011) & (±0.012) & (±0.006) & (±0.015) & (±0.006) & (±0.007) & (±0.007) & (±0.018) &  (±0.011)\\

cardiotocography & 0.788 & 0.735 & 0.707 & 0.730 & 0.750 & 0.767 & 0.691 & 0.697 & 0.774 & 0.733 & 0.738 & 0.712 & 0.678 & 0.757 & 0.767 & 0.630 \\
 & (±0.012) & (±0.013) & (±0.016) & (±0.008) & (±0.008) & (±0.025) & (±0.022) & (±0.011) & (±0.016) & (±0.016) & (±0.016) & (±0.017) & (±0.009) & (±0.021) & (±0.025) & (±0.018) \\

census & 0.354 & 0.168 & 0.335 & 0.136 & 0.153 & 0.346 & 0.411 & 0.304 & 0.395 & 0.352 & 0.281 & 0.308 & 0.371 & 0.315 & 0.348 & 0.222 \\
 & (±0.005) & (±0.003) & (±0.003) & (±0.002) & (±0.001) & (±0.060) & (±0.015) & (±0.003) & (±0.004) & (±0.006) & (±0.003) & (±0.005) & (±0.005) & (±0.012) & (±0.022) & (±0.010) \\

churn & 0.520 & 0.395 & 0.420 & 0.407 & 0.486 & 0.477 & 0.464 & 0.430 & 0.505 & 0.563 & 0.527 & 0.471 & 0.406 & 0.463 & 0.463 & 0.429 \\
 & (±0.010) & (±0.007) & (±0.003) & (±0.005) & (±0.014) & (±0.071) & (±0.048) & (±0.002) & (±0.034) & (±0.005) & (±0.003) & (±0.010) & (±0.005) & (±0.025) & (±0.005) & (±0.016) \\

cirrhosis & 0.836 & 0.850 & 0.850 & 0.866 & 0.834 & 0.819 & 0.883 & 0.792 & 0.845 & 0.818 & 0.836 & 0.826 & 0.835 & 0.841 & 0.822 & 0.824 \\
 & (±0.014) & (±0.014) & (±0.013) & (±0.012) & (±0.016) & (±0.018) & (±0.014) & (±0.020) & (±0.013) & (±0.024) & (±0.028) & (±0.018) & (±0.013) & (±0.016) & (±0.016) & (±0.017) \\

covertype & 0.871 & 0.802 & 0.874 & 0.320 & 0.304 & 0.825 & 0.468 & 0.743 & 0.915 & 0.890 & 0.940 & 0.914 & 0.923 & 0.880 & 0.781 & 0.654 \\
 & (±0.011) & (±0.011) & (±0.004) & (±0.023) & (±0.010) & (±0.031) & (±0.114) & (±0.016) & (±0.012) & (±0.026) & (±0.003) & (±0.009) & (±0.015) & (±0.027) & (±0.062) & (±0.020) \\

credit & 0.610 & 0.412 & 0.556 & 0.483 & 0.547 & 0.540 & 0.559 & 0.410 & 0.600 & 0.575 & 0.576 & 0.583 & 0.566 & 0.545 & 0.525 & 0.352 \\
 & (±0.005) & (±0.006) & (±0.014) & (±0.003) & (±0.005) & (±0.033) & (±0.012) & (±0.008) & (±0.004) & (±0.008) & (±0.027) & (±0.003) & (±0.003) & (±0.006) & (±0.037) & (±0.018) \\

equip & 0.972 & 0.971 & 0.972 & 0.950 & 0.970 & 0.965 & 0.969 & 0.941 & 0.971 & 0.969 & 0.967 & 0.954 & 0.970 & 0.970 & 0.966 & 0.972 \\
 & (±0.000) & (±0.001) & (±0.000) & (±0.001) & (±0.001) & (±0.001) & (±0.001) & (±0.002) & (±0.001) & (±0.000) & (±0.001) & (±0.003) & (±0.000) & (±0.001) & (±0.004) & (±0.002) \\

gallstone & 0.667 & 0.702 & 0.691 & 0.637 & 0.630 & 0.724 & 0.642 & 0.727 & 0.710 & 0.721 & 0.775 & 0.746 & 0.649 & 0.744 & 0.733 & 0.580 \\
 & (±0.052) & (±0.036) & (±0.046) & (±0.008) & (±0.036) & (±0.031) & (±0.035) & (±0.023) & (±0.037) & (±0.038) & (±0.009) & (±0.032) & (±0.036) & (±0.035) & (±0.022) & (±0.027) \\

glass & 0.920 & 0.942 & 0.894 & 0.869 & 0.878 & 0.918 & 0.850 & 0.919 & 0.907 & 0.923 & 0.928 & 0.900 & 0.881 & 0.917 & 0.896 & 0.808 \\
 & (±0.027) & (±0.021) & (±0.038) & (±0.049) & (±0.035) & (±0.041) & (±0.043) & (±0.035) & (±0.043) & (±0.036) & (±0.035) & (±0.029) & (±0.029) & (±0.042) & (±0.038) & (±0.024) \\

glioma & 0.761 & 0.673 & 0.785 & 0.706 & 0.703 & 0.753 & 0.712 & 0.718 & 0.801 & 0.781 & 0.741 & 0.863 & 0.684 & 0.802 & 0.702 & 0.688 \\
 & (±0.013) & (±0.025) & (±0.007) & (±0.014) & (±0.016) & (±0.023) & (±0.038) & (±0.016) & (±0.009) & (±0.010) & (±0.024) & (±0.006) & (±0.011) & (±0.008) & (±0.034) & (±0.022) \\

quasar & 0.918 & 0.949 & 0.952 & 0.758 & 0.863 & 0.707 & 0.891 & 0.932 & 0.937 & 0.860 & 0.932 & 0.926 & 0.776 & 0.927 & 0.850 & 0.936 \\
 & (±0.006) & (±0.009) & (±0.002) & (±0.022) & (±0.025) & (±0.191) & (±0.016) & (±0.002) & (±0.010) & (±0.036) & (±0.003) & (±0.005) & (±0.020) & (±0.006) & (±0.040) & (±0.013) \\

seismic & 0.248 & 0.168 & 0.257 & 0.247 & 0.204 & 0.256 & 0.261 & 0.231 & 0.253 & 0.246 & 0.236 & 0.239 & 0.253 & 0.249 & 0.246 & 0.283 \\
 & (±0.004) & (±0.005) & (±0.006) & (±0.010) & (±0.004) & (±0.005) & (±0.006) & (±0.009) & (±0.006) & (±0.005) & (±0.012) & (±0.007) & (±0.006) & (±0.016) & (±0.009) & (±0.009) \\

stroke & 0.228 & 0.116 & 0.227 & 0.214 & 0.179 & 0.178 & 0.244 & 0.153 & 0.247 & 0.202 & 0.171 & 0.185 & 0.217 & 0.242 & 0.206 & 0.163 \\
 & (±0.011) & (±0.004) & (±0.008) & (±0.009) & (±0.006) & (±0.007) & (±0.013) & (±0.007) & (±0.012) & (±0.007) & (±0.007) & (±0.010) & (±0.013) & (±0.010) & (±0.004) & (±0.010) \\

vertebral & 0.545 & 0.513 & 0.446 & 0.463 & 0.485 & 0.584 & 0.421 & 0.518 & 0.504 & 0.597 & 0.636 & 0.605 & 0.385 & 0.582 & 0.461 & 0.551 \\
 & (±0.032) & (±0.021) & (±0.021) & (±0.013) & (±0.010) & (±0.049) & (±0.121) & (±0.013) & (±0.012) & (±0.030) & (±0.044) & (±0.028) & (±0.002) & (±0.117) & (±0.037) & (±0.028) \\

wbc & 0.970 & 0.962 & 0.962 & 0.956 & 0.959 & 0.974 & 0.856 & 0.922 & 0.962 & 0.955 & 0.761 & 0.936 & 0.781 & 0.955 & 0.950 & 0.827 \\
 & (±0.007) & (±0.007) & (±0.008) & (±0.009) & (±0.010) & (±0.005) & (±0.031) & (±0.013) & (±0.011) & (±0.007) & (±0.028) & (±0.019) & (±0.014) & (±0.010) & (±0.025) & (±0.019) \\

wine & 0.933 & 0.957 & 0.960 & 0.980 & 0.967 & 0.959 & 0.505 & 0.889 & 0.954 & 0.952 & 0.981 & 0.967 & 0.714 & 0.969 & 0.926 & 0.874 \\
 & (±0.022) & (±0.027) & (±0.021) & (±0.010) & (±0.015) & (±0.021) & (±0.039) & (±0.051) & (±0.022) & (±0.033) & (±0.008) & (±0.019) & (±0.062) & (±0.019) & (±0.021) & (±0.023) \\

yeast & 0.427 & 0.311 & 0.369 & 0.435 & 0.384 & 0.359 & 0.370 & 0.299 & 0.420 & 0.390 & 0.351 & 0.384 & 0.361 & 0.455 & 0.381 & 0.369 \\
 & (±0.027) & (±0.018) & (±0.004) & (±0.055) & (±0.022) & (±0.030) & (±0.102) & (±0.019) & (±0.029) & (±0.013) & (±0.018) & (±0.045) & (±0.008) & (±0.051) & (±0.061) & (±0.040) \\




\bottomrule
\end{tabular}
}
\end{table}
% \end{sidewaystable}
