# Supplementary material for: ReTabAD: A Benchmark for Restoring Semantic Context in Tabular Anomaly Detection
Source: arXiv:2510.02060 source file (2026-05-28)
Supplement: Supplementary file 4 [file auroc_full_backup.tex]

\begin{table}[htbp]
\centering
\scriptsize
\caption{AUROC Performance across all baselines.}
\label{tab:auroc_results2}
\resizebox{\textwidth}{!}{%
\begin{tabular}{lcccccccccccccccc}
\toprule
Dataset & OCSVM & LOF & KNN & IForest & PCA & DeepSVDD & REPEN & RDP & RCA & GOAD & NeuTraL & SLAD & DIF & MCM & DRL & AnoLLM \\
\midrule
\midrule
automobile & 0.645 & 0.688 & 0.656 & 0.648 & 0.497 & 0.845 & 0.611 & 0.774 & 0.679 & 0.676 & 0.810 & 0.780 & 0.647 & 0.801 & 0.762 & 0.624 \\
 & (±0.025) & (±0.029) & (±0.015) & (±0.034) & (±0.028) & (±0.030) & (±0.059) & (±0.017) & (±0.025) & (±0.065) & (±0.012) & (±0.030) & (±0.023) & (±0.013) & (±0.066) & (±0.021) \\

backdoor & 0.876 & 0.702 & 0.934 & 0.888 & 0.822 & 0.800 & 0.856 & 0.897 & 0.915 & 0.889 & 0.948 & 0.935 & 0.973 & 0.961 & 0.902 & 0.885 \\
 & (±0.004) & (±0.008) & (±0.004) & (±0.004) & (±0.003) & (±0.116) & (±0.013) & (±0.001) & (±0.003) & (±0.007) & (±0.001) & (±0.001) & (±0.002) & (±0.003) & (±0.017) & (±0.010) \\

campaign & 0.700 & 0.669 & 0.754 & 0.732 & 0.750 & 0.721 & 0.697 & 0.693 & 0.722 & 0.740 & 0.760 & 0.717 & 0.677 & 0.761 & 0.737 & 0.738 \\
 & (±0.004) & (±0.005) & (±0.007) & (±0.006) & (±0.003) & (±0.014) & (±0.010) & (±0.010) & (±0.010) & (±0.002) & (±0.008) & (±0.002) & (±0.004) & (±0.005) & (±0.018) & (±0.012) \\

cardiotocography & 0.868 & 0.826 & 0.780 & 0.830 & 0.840 & 0.813 & 0.759 & 0.766 & 0.858 & 0.788 & 0.791 & 0.764 & 0.740 & 0.843 & 0.847 & 0.735 \\
 & (±0.006) & (±0.010) & (±0.011) & (±0.006) & (±0.005) & (±0.015) & (±0.035) & (±0.008) & (±0.005) & (±0.012) & (±0.016) & (±0.018) & (±0.007) & (±0.012) & (±0.019) & (±0.014) \\

census & 0.647 & 0.596 & 0.738 & 0.620 & 0.627 & 0.712 & 0.811 & 0.717 & 0.745 & 0.708 & 0.686 & 0.687 & 0.726 & 0.729 & 0.728 & 0.737 \\
 & (±0.001) & (±0.002) & (±0.001) & (±0.009) & (±0.002) & (±0.048) & (±0.007) & (±0.002) & (±0.002) & (±0.002) & (±0.002) & (±0.002) & (±0.005) & (±0.007) & (±0.036) & (±0.009) \\

churn & 0.651 & 0.465 & 0.532 & 0.506 & 0.579 & 0.573 & 0.546 & 0.523 & 0.616 & 0.683 & 0.651 & 0.571 & 0.494 & 0.580 & 0.553 & 0.557 \\
 & (±0.007) & (±0.007) & (±0.003) & (±0.010) & (±0.023) & (±0.071) & (±0.058) & (±0.004) & (±0.030) & (±0.006) & (±0.004) & (±0.014) & (±0.005) & (±0.024) & (±0.012) & (±0.018) \\

cirrhosis & 0.823 & 0.843 & 0.843 & 0.849 & 0.822 & 0.807 & 0.876 & 0.795 & 0.834 & 0.816 & 0.831 & 0.810 & 0.820 & 0.830 & 0.814 & 0.850 \\
 & (±0.012) & (±0.013) & (±0.012) & (±0.013) & (±0.017) & (±0.018) & (±0.010) & (±0.023) & (±0.012) & (±0.022) & (±0.022) & (±0.018) & (±0.011) & (±0.020) & (±0.012) & (±0.015) \\

covertype & 0.998 & 0.980 & 0.991 & 0.968 & 0.976 & 0.971 & 0.986 & 0.992 & 0.998 & 0.998 & 0.998 & 0.999 & 0.998 & 0.998 & 0.995 & 0.990 \\
 & (±0.000) & (±0.003) & (±0.000) & (±0.003) & (±0.001) & (±0.007) & (±0.006) & (±0.001) & (±0.000) & (±0.000) & (±0.000) & (±0.000) & (±0.000) & (±0.000) & (±0.002) & (±0.003) \\

credit & 0.717 & 0.590 & 0.692 & 0.639 & 0.684 & 0.638 & 0.661 & 0.593 & 0.702 & 0.682 & 0.690 & 0.691 & 0.689 & 0.671 & 0.680 & 0.495 \\
 & (±0.003) & (±0.007) & (±0.007) & (±0.003) & (±0.003) & (±0.039) & (±0.012) & (±0.009) & (±0.002) & (±0.005) & (±0.016) & (±0.002) & (±0.002) & (±0.004) & (±0.020) & (±0.019) \\

equip & 0.987 & 0.987 & 0.987 & 0.980 & 0.986 & 0.984 & 0.986 & 0.973 & 0.986 & 0.983 & 0.985 & 0.981 & 0.987 & 0.986 & 0.984 & 0.986 \\
 & (±0.000) & (±0.000) & (±0.000) & (±0.000) & (±0.000) & (±0.000) & (±0.000) & (±0.001) & (±0.000) & (±0.001) & (±0.000) & (±0.001) & (±0.000) & (±0.001) & (±0.001) & (±0.002) \\

gallstone & 0.671 & 0.704 & 0.702 & 0.650 & 0.637 & 0.731 & 0.621 & 0.725 & 0.720 & 0.734 & 0.780 & 0.758 & 0.649 & 0.757 & 0.745 & 0.574 \\
 & (±0.047) & (±0.032) & (±0.040) & (±0.021) & (±0.026) & (±0.020) & (±0.049) & (±0.029) & (±0.033) & (±0.034) & (±0.019) & (±0.028) & (±0.026) & (±0.034) & (±0.029) & (±0.028) \\

glass & 0.959 & 0.974 & 0.953 & 0.944 & 0.938 & 0.963 & 0.936 & 0.965 & 0.959 & 0.967 & 0.968 & 0.952 & 0.936 & 0.966 & 0.949 & 0.907 \\
 & (±0.010) & (±0.010) & (±0.014) & (±0.016) & (±0.011) & (±0.012) & (±0.018) & (±0.011) & (±0.014) & (±0.011) & (±0.010) & (±0.011) & (±0.012) & (±0.012) & (±0.013) & (±0.016) \\

glioma & 0.725 & 0.711 & 0.787 & 0.722 & 0.715 & 0.766 & 0.727 & 0.739 & 0.787 & 0.772 & 0.784 & 0.886 & 0.686 & 0.790 & 0.764 & 0.708 \\
 & (±0.012) & (±0.016) & (±0.006) & (±0.013) & (±0.012) & (±0.012) & (±0.039) & (±0.015) & (±0.008) & (±0.009) & (±0.013) & (±0.005) & (±0.012) & (±0.009) & (±0.040) & (±0.022) \\

quasar & 0.930 & 0.966 & 0.969 & 0.915 & 0.894 & 0.804 & 0.931 & 0.953 & 0.950 & 0.901 & 0.954 & 0.952 & 0.793 & 0.950 & 0.897 & 0.961 \\
 & (±0.008) & (±0.009) & (±0.004) & (±0.007) & (±0.013) & (±0.135) & (±0.014) & (±0.004) & (±0.012) & (±0.014) & (±0.006) & (±0.009) & (±0.042) & (±0.007) & (±0.024) & (±0.014) \\

seismic & 0.710 & 0.615 & 0.741 & 0.710 & 0.671 & 0.729 & 0.739 & 0.719 & 0.729 & 0.717 & 0.716 & 0.727 & 0.736 & 0.716 & 0.714 & 0.741 \\
 & (±0.002) & (±0.007) & (±0.005) & (±0.006) & (±0.003) & (±0.015) & (±0.005) & (±0.006) & (±0.005) & (±0.003) & (±0.007) & (±0.006) & (±0.005) & (±0.019) & (±0.016) & (±0.011) \\

stroke & 0.716 & 0.625 & 0.732 & 0.679 & 0.678 & 0.722 & 0.745 & 0.674 & 0.764 & 0.709 & 0.703 & 0.678 & 0.705 & 0.753 & 0.727 & 0.687 \\
 & (±0.004) & (±0.022) & (±0.005) & (±0.003) & (±0.004) & (±0.005) & (±0.017) & (±0.009) & (±0.011) & (±0.002) & (±0.005) & (±0.007) & (±0.007) & (±0.005) & (±0.025) & (±0.010)\\

vertebral & 0.638 & 0.540 & 0.469 & 0.500 & 0.524 & 0.581 & 0.340 & 0.551 & 0.566 & 0.687 & 0.697 & 0.679 & 0.340 & 0.615 & 0.477 & 0.597 \\
 & (±0.043) & (±0.021) & (±0.038) & (±0.019) & (±0.013) & (±0.062) & (±0.100) & (±0.018) & (±0.020) & (±0.037) & (±0.040) & (±0.020) & (±0.008) & (±0.128) & (±0.042) & (±0.014) \\

wbc & 0.969 & 0.960 & 0.961 & 0.961 & 0.960 & 0.969 & 0.879 & 0.924 & 0.964 & 0.947 & 0.785 & 0.938 & 0.679 & 0.957 & 0.954 & 0.871 \\
 & (±0.006) & (±0.006) & (±0.006) & (±0.004) & (±0.006) & (±0.005) & (±0.026) & (±0.010) & (±0.007) & (±0.009) & (±0.024) & (±0.023) & (±0.016) & (±0.006) & (±0.010) & (±0.031) \\

wine & 0.957 & 0.974 & 0.976 & 0.987 & 0.980 & 0.974 & 0.657 & 0.939 & 0.973 & 0.973 & 0.988 & 0.980 & 0.760 & 0.979 & 0.958 & 0.933 \\
 & (±0.012) & (±0.014) & (±0.012) & (±0.006) & (±0.007) & (±0.011) & (±0.053) & (±0.032) & (±0.011) & (±0.009) & (±0.002) & (±0.010) & (±0.033) & (±0.012) & (±0.012) & (±0.020) \\

yeast & 0.875 & 0.803 & 0.831 & 0.838 & 0.861 & 0.820 & 0.826 & 0.786 & 0.866 & 0.836 & 0.841 & 0.846 & 0.815 & 0.856 & 0.841 & 0.809 \\
 & (±0.008) & (±0.010) & (±0.007) & (±0.014) & (±0.009) & (±0.015) & (±0.049) & (±0.004) & (±0.008) & (±0.007) & (±0.009) & (±0.019) & (±0.004) & (±0.014) & (±0.033) & (±0.018) \\



\bottomrule
\end{tabular}
}
\end{table}
